# Supplementary material for: Bundle gerbes and the Weyl map
Source: arXiv:1910.01776 source file (2019-10-03)
Supplement: Supplementary file 1 [file appendix.tex]

%!TEX root = ../thesis.tex
\chapter{second appendix\label{app:the_second}}
